# Supplementary material for: Sharp global convergence guarantees for iterative nonconvex optimization: A Gaussian process perspective
Source: arXiv:2109.09859 source file (2021-09-20)
Supplement: Supplementary file 2 [file aux-PR.tex]

%!TEX root = ../../convergence-gordon.tex

\section{Auxiliary proofs for phase retrieval}

\subsection{Population update: Proof of Fact~\ref{prop:Pop-PR}}

Let us begin by restating the population update.
\begin{align*}
\xipop = 1 - \frac{1}{\pi}(2\alpha - \sin(2\alpha))  \qquad \text{ and } \qquad \sigmapop = \frac{2}{\pi}\sin^2(\alpha). 
\end{align*}
We refer to these as the $F$ and $G$ maps respectively and let $\mathcal{S}_{pop}$ denote the population state evolution operator. The fact is an immediate consequence of the following two lemmas, which we state and prove below.
\begin{lemma}
If $\nu \in \GPR$, then $\mathcal{S}_{pop}(\nu) \in \GPR$.
\end{lemma}
\begin{proof}
Clearly, we have $F \lor G \leq 1$. Since the $\xipop$ update coincides with the Gordon update $\xigordon$, equation~\eqref{eq:rec-sqbound} yields that $F^2 + G^2 \geq 0.9$ provided $\alpha \leq \tan^{-1}(1/5)$. Finally, since $G \leq 2 \cdot (0.2)^2 / \pi$ and $F \geq 0.9$ for all $\alpha \leq 0.2$, we have $G/F \leq 1/5$, as desired.
\end{proof}

\begin{lemma} 
For each $\nu = (\xi, \sigma) \in \GPR$, we have
\begin{align*}
\DeltaSE(\mathcal{S}_{pop}(\nu)) \leq[\DeltaSE(\nu)]^{2} \quad \text{ and } \quad \DeltaSE(\mathcal{S}^2_{pop}(\nu)) \geq \frac{1}{\sqrt{20}} \cdot [\DeltaSE(\mathcal{S}_{pop}(\nu))]^{2}.
\end{align*}
\end{lemma}
\begin{proof}
Beginning with the upper bound, recall that any $(\xi, \sigma) \in \GPR$ satisfies $\xi \geq 0.93$ and $\xi^3 \geq 0.6$. We also have $\alpha \leq \sigma/ \xi \leq 1/5$. The $\sigmapop$ update can be bounded as
\begin{align*}
[G(\xi, \sigma)]^2 &\leq \frac{4}{\pi^2} \alpha^4
\end{align*}
On the other hand, Equation~\eqref{eq:xi-ineq} yields
\begin{align*}
(1 - F(\xi, \sigma))^2 &= \frac{1}{\pi^2} (2 \alpha - \sin(2\alpha))^2 \leq \frac{16}{9 \pi^2} \alpha^6.
\end{align*}
Putting together the pieces, we have
\begin{align*}
[\DeltaSE(\mathcal{S}_{pop}(\nu))]^2 = [G(\xi, \sigma)]^2 + (1 - F(\xi, \sigma))^2 \leq \sigma^4 \leq \left\{ \sigma^2 + (1 - \xi)^2 \right\}^{2},
\end{align*}
where the first inequality is a result of noting that $\alpha \leq \sigma / \xi$ and $\xi \geq 0.6$.


Moving now to the lower bound, let us compute two steps of the Gordon update, letting $F_{+} = F^2(\xi, \sigma)$ and $G_+ = G^2(\xi, \sigma)$. Analogously, we let $F = F(\xi, \sigma)$ and $G = G(\xi, \sigma)$, and use $\alpha_+ = \tan^{-1} (G/F)$ to denote the angle after one step of the Gordon update. Recall that $\tan \alpha = \sigma/\xi$. We have
\begin{align*}
G_{+}^2 = \frac{4}{\pi^2} \cdot \sin^4 \alpha_+ = \frac{4G^4}{\pi^2(F^2 + G^2)^2} \geq \frac{4 \pi^2}{(\pi^2 + 4)^2} \cdot G^4 > \frac{G^4}{5},
\end{align*}
where the penultimate inequality uses the fact that $F \leq 1$ and $G \leq 2/\pi$, guaranteed by one step of the Gordon update. Turning now to the $F_+$ component, we have
\begin{align*}
\pi^2 (1 - F_+)^2  = (2 \alpha_+ - \sin(2\alpha_+))^2 \geq \frac{G^6}{64}.
\end{align*}
At the same time, we have $(1 - F)^4 \leq \frac{1}{16 \pi^2} G^6$, since $\alpha_+ \leq 0.2$.
Putting together the pieces yields
\begin{align*}
G_{+}^2 + (1 - F_+)^2 &\geq \frac{G^4}{5} + \frac{G^6}{64\pi^2} \geq \frac{G^4}{5} + \frac{(1 - F)^4}{4} \geq \frac{1}{20} \cdot \left\{ G^2 + (1 - F)^2 \right\}^{2},
\end{align*}
where the last step follows because $(A + B)^{\kappa} \leq 2^{\kappa} (A^\kappa + B^{\kappa})$ for any positive scalars $(A, B)$ and $\kappa \geq 1$.
\end{proof}


\begin{remark}
The claimed quadratic convergence holds in a region much larger than the good region $\GPR$. Indeed, it is easy to show that $\tan^{-1} (G/F) \leq \frac{2}{\pi} \cdot \left( \tan^{-1} (\sigma / \xi) \right)^2$, showing that the \emph{angle} converges quadratically fast, globally for any $\alpha < \pi/2$.
\end{remark}

\subsection{AM update}

In this section, we prove Lemma~\ref{lem:Gordon-SE-AM-PR}, and also provide a technical lemma regarding Taylor expansions of the Gordon state evolution maps~\eqref{eq:Gordon-AM-PR-restated}. The latter lemma is used in the proof of Theorem~\ref{thm:AM-PR}(b).

\subsubsection{Proof of Lemma~\ref{lem:Gordon-SE-AM-PR}}

\apcomment{Insert after Gordon structure/notation stabilizes.}

\iffalse
\subsubsection{Structural properties of Gordon state evolution}

The following lemma collects some elementary properties of the Gordon recursion for the AM update.
\begin{lemma}\label{lem:Gordon-AM-struct}
(a) Suppose $\delta \geq 10$ and that $s^2 /\delta \leq c$ for a sufficiently small universal constant $c$. For all $(\sigma, \xi)$ pairs with $1/2 \leq \xi/\sigma \leq 5$, we have
\[
\frac{G(\xi, \sigma)}{F(\xi, \sigma)} \leq \sqrt{\frac{2}{3}} \cdot \frac{\sigma}{\xi}.
\]


(b) Suppose $\delta \geq 10$ and $s = 0$. For all $(\sigma, \xi)$ pairs with $\sigma/\xi \in [0, \infty)$, we have
\[
\frac{G(\xi, \sigma)}{F(\xi, \sigma)} \leq \sqrt{\frac{2}{3}} \cdot \frac{\sigma}{\xi}.
\]

(c) For all $(\sigma, \xi)$ pairs with $(\sigma/\xi)^3 \leq \frac{3\pi}{4}$, we have
\[
[F(\xi, \sigma)]^2  + [G(\xi, \sigma)]^2  \geq [F(\xi, \sigma)]^2 \geq \left(1 - \frac{4}{3\pi} \left( \sigma/\xi \right)^3 \right)^2.
\]
\end{lemma}
\begin{proof}[Proof of Lemma~\ref{lem:Gordon-AM-struct}(b)]
The proof of this lemma involves showing some properties about the square of the ratio $\frac{G(\xi, \sigma)}{F(\xi, \sigma)} \div \frac{\sigma}{\xi}$. Denote the square of this ratio by a function $H_\delta$ of the angle, and note that the Gordon recursion yields
\[
(\delta - 1) \cdot H_{\delta}(\alpha) = \frac{\cot^2 \alpha}{(\pi - 2 \alpha + \sin (2\alpha))^2} \cdot \left\{ 4 (\delta - 2) \sin^4 \alpha + \pi^2 - (\pi - 2 \alpha + \sin (2\alpha))^2 \right\}.
\]
We now split the proof into two cases:

\noindent \underline{Case $\alpha \in [0, \pi/4]$:} In this case, we make use of the easily-verified bounds
\begin{align*}
\cot^2 \alpha &\leq \alpha^{-2}, \\
(\pi - 2\alpha + \sin(2\alpha))^2 &\geq (1 + \pi/2)^2, \qquad \text{ and } \\
4(\delta - 2) \sin^4 \alpha + \pi^2 - (\pi - 2\alpha + \sin(2\alpha))^2 &\leq 4(\delta - 2) \alpha^4 + 2(2\alpha - \sin(2\alpha)) \\
& \leq 4(\delta - 2) \alpha^4 + \frac{8}{3} \alpha^3.
\end{align*}
Substituting above yields
\begin{align*}
(\delta - 1) \cdot H_{\delta}(\alpha) \leq \frac{4(\delta - 2) \alpha^2 + \frac{8}{3} \alpha}{(1 + \pi/2)^2} \leq \frac{\pi^2 (\delta - 2) }{(\pi + 2)^2}  + \frac{8\pi}{3(\pi + 2)^2} \leq 0.37 \cdot (\delta - 1).
\end{align*}
The last inequality follows by assumption $\delta \geq 10$.

\noindent \underline{Case $\alpha \in [\pi/4, \pi/2)$:} Let $\beta = \pi/2 - \alpha$, and note that for all $\beta \in (0, \pi/4)$, we have
\begin{align*}
\tan^2 \beta &\leq \frac{16}{\pi^2} \cdot \beta^2 \\
(2 \beta + \sin(2 \beta))^2 &\geq 4 (1 + 2/\pi)^2 \beta^2, \text{ and } \\
4(\delta - 2) \cos^4 \beta + \pi^2 - (2 \beta + \sin(2 \beta))^2 &\leq 4(\delta - 2) + \pi^2.
\end{align*}
Substituting above yields
\begin{align*}
(\delta - 1) \cdot H_{\delta}(\alpha) \leq \frac{16(\delta - 2)}{(\pi+2)^2} + \frac{\pi^2}{10} \leq 0.65 \cdot (\delta - 1).
\end{align*}
Once again, the last inequality holds provided $\delta \geq 10$.
% Old proof, new one is cleaner.
% The proof will by proceed by first showing an analogous result for the Gordon update, and then translating that to the empirics via Lemma~\ref{lem:noise bound}. We have 
% \begin{align*}
% \frac{F(\xi, \sigma)}{G(\xi, \sigma)} &\geq \left( 1 - \frac{1}{\pi} (2 \alpha - \sin(2\alpha)) \right) \div \left( \sqrt{\frac{\delta - 2}{\delta - 1}} \cdot \frac{2}{\pi} \sin^2 \alpha \right) \\
% &\geq \frac{\tan^{-1} (\xi/\sigma)}{\sin^2 \alpha} \\
% &\stackrel{(i)}{\geq}  \frac{\xi}{\sqrt{\xi^2 + \sigma^2}} \cdot \frac{\xi^2 + \sigma^2}{\sigma^2} = \frac{\xi}{\sigma} \cdot \sqrt{1 + \left( \frac{\xi}{\sigma} \right)^2 } > \frac{4}{3} \cdot \frac{\xi}{\sigma}.
% \end{align*}
% In step (i), we have used the fact that $x \geq \sin x$.
\end{proof}


\begin{proof}[Proof of Lemma~\ref{lem:Gordon-AM-struct}(c)]
The first inequality is trivial; to prove the second inequality, note that since $\sin x \geq x - x^3/6$, we have $2\alpha - \sin(2 \alpha) \leq \frac{4}{3} \alpha^3$. Moreover, when $(\sigma/\xi)^3 \leq \frac{3 \pi}{4}$, we also have $1 - \frac{4}{3\pi} \alpha^3 \geq 1 - \frac{4}{3\pi} \tan^3 \alpha \geq 0$. Consequently, for all such $\alpha$, we have
\begin{align*}
[F(\xi, \sigma)]^2 = \left( 1 - \frac{1}{\pi} (2\alpha - \sin(2 \alpha)) \right)^2 \geq  \left( 1 - \frac{4}{3\pi} (\sigma/\xi)^3 \right)^2,
\end{align*}
completing the proof.
\end{proof}
\fi

\subsubsection{Perturbation lemma for Gordon state evolution maps}

The first result is for the Gordon state evolution corresponding to AM~\eqref{eq:Gordon-AM-PR}. Recall that $F$ and $G$ denote the two Gordon maps $\xigordon$ and $\sigmagordon$, respectively.

\begin{lemma}[Local $\ell_\infty$ perturbation] \label{lem:Gordon-pert}
Suppose the pair $(\xi, \sigma)$ satisfies $\xi/\sigma \geq 5$ and $\xi^2 + \sigma^2 \geq 0.9$. Also suppose that $\delta \geq 42$. There is a universal constant $\tau \in (0, 1)$ such that for all pairs of positive scalars $(\xi', \sigma')$ satisfying $|\xi' - \xi| \lor | \sigma' - \sigma| \leq 1/200$, we have
\begin{align*}
|F(\xi, \sigma) - F(\xi', \sigma')| &\leq (1 - \tau) \left( | \xi' - \xi| \lor |\sigma' - \sigma| \right) \text{ and } \\
|G(\xi, \sigma) - G(\xi', \sigma')| &\leq (1 - \tau) \left( | \xi' - \xi| \lor |\sigma' - \sigma| \right).
\end{align*}
\end{lemma}

\begin{proof}
The perturbation result is proved by Taylor expansions, and this requires the computation of higher order derivatives. Note that we have $F(\xi, \sigma) = \Phi(\alpha(\xi, \sigma))$ and $G(\xi, \sigma) = \Gamma(\alpha(\xi, \sigma))$ for two functions $\Phi$ and $\Gamma$. By chain rule, we have
\begin{align*}
\nabla F(\xi, \sigma) = \Phi'(\alpha) \cdot \nabla \alpha(\xi, \sigma) \quad \text{ and } \quad \nabla G(\xi, \sigma) = \Gamma'(\alpha) \cdot \nabla \alpha(\xi, \sigma).
\end{align*}
Since $\alpha = \tan^{-1} (\sigma/\xi)$, we also have $\nabla \alpha(\xi, \sigma) = \left( -\frac{-\sigma}{\xi^2 + \sigma^2}, -\frac{\xi}{\xi^2 + \sigma^2} \right)$; by the Cauchy-Schwarz inequality, this has $\ell_1$ norm bounded as
\begin{align*}
\| \nabla \alpha(\xi, \sigma) \|_1 \leq \frac{\xi + \sigma}{\xi^2 + \sigma^2} \leq \sqrt{\frac{2}{\xi^2 + \sigma^2}}.
\end{align*}
For each $u \in [0, 1]$, let $\xi^u = u \xi + (1 - u)\xi'$ and $\sigma^u = u \sigma + (1 - u)\sigma'$. Also, let $\beta^u = (\xi^u, \sigma^u)$ and $\beta = \beta^0 = (\xi, \sigma)$ for convenience, and define $\nu = (\xi, \sigma) - (\xi', \sigma')$. By Young's inequality, the following relation holds for each $\eta > 0$ and $u \in [0, 1]$:
\begin{align*}
\| \beta^u \|_2^2 \geq \frac{1}{1 + \eta} \cdot \| \beta \|_2^2 - \frac{1}{\eta} \| \beta^u - \beta \|_2^2 \geq \frac{0.9}{1 + \eta} - \frac{1}{\eta} \| \nu \|_2^2.
\end{align*}
By setting $\eta = 1/200$ and noting that $\| \nu \|_2^2 \leq 0.2 \times 10^{-4}$, we have $\| \beta^u \|_2^2 \geq 0.88$ for all $u \in [0, 1]$.
If $(\xi, \sigma)$ satisfy $\xi/\sigma \geq 5$ and $\xi^2 + \sigma^2 \geq 0.9$, then we have $\xi \geq 0.93$. Consequently, for all $u \in [0, 1]$, we have
\begin{align*}
\frac{\sigma^u}{\xi^u} \leq \frac{\sigma + 1/200}{\xi - 1/200} \leq 0.206.
\end{align*}

Finally, some calculation yields that $\Phi'(\alpha) = \frac{4}{\pi} \sin^2 \alpha$, so that $\Phi'(\alpha^u) = \frac{4}{\pi} \frac{\sigma^2 / \xi^2}{1 + \sigma^2 / \xi^2} \leq \frac{1}{6\pi}$ for all $u \in [0, 1]$.
Also note that $\Gamma(\alpha) = \sqrt{S(\alpha)}$ for 
\[
S(\alpha) = \frac{4}{\pi^2} \cdot \frac{\delta - 2}{\delta - 1} \cdot \sin^4(\alpha) + \frac{1}{\delta - 1}\left(1 - (1 - \frac{1}{\pi}(2\alpha - \sin(2\alpha)))^2 \right)
\]
whence
\begin{align*}
|\Gamma'(\alpha)| = \frac{|S'(\alpha)|}{\sqrt{S(\alpha)}} \leq \frac{ \left| \frac{16}{\pi^2} \sin^3 \alpha + \frac{2}{\delta - 2} \cdot \frac{4}{\pi} \cdot \sin^2 \alpha \right|}{ \frac{2}{\pi} \sin^2 \alpha} \leq \frac{8}{\pi} \sin \alpha + \frac{1}{10},
\end{align*}
where the final step holds for $\delta \geq 42$. Thus, for all $u \in [0, 1]$, we have $|\Gamma'(\alpha^u)| \leq \frac{8}{\pi} \cdot \frac{1}{\sqrt{24}} + 1/10 \leq 0.62$.

Since both $F$ and $G$ are continuously differentiable provided their argument is non-zero, for any tuple of strictly positive scalars $(\xi, \xi', \sigma, \sigma')$, we have the Taylor expansion
\begin{align*}
F(\xi', \sigma') &= F(\xi, \sigma) + \inprod{ \nu}{\nabla F(\xi^u, \sigma^{u})} \text{ and } \\
G(\xi', \sigma') &= G(\xi, \sigma) + \inprod{ \nu}{\nabla G(\xi^{u'}, \sigma^{u'})},
\end{align*}
for some $u, u' \in [0, 1]$. From the calculations above, we obtain
\begin{align}
\begin{split} \label{eq:Fmap-AMPR}
\sup_{0 \leq u \leq 1}\| \nabla F(\xi^u, \sigma^{u}) \|_1 &\leq \frac{1}{6\pi} \cdot \sqrt{\frac{2}{0.88}} \leq 1/10 \text{ and } \\
\sup_{0 \leq u \leq 1}\| \nabla G(\xi^u, \sigma^{u}) \|_1 &\leq 0.62 \cdot \sqrt{\frac{2}{0.88}} \leq 0.98,
\end{split}
\end{align}
and using Holder's inequality completes the proof.
\end{proof}
% Need (a) ratio lemmas, (b) xi lemmas, (c) Taylor lemmas for the non-linear portion of recursion.

\subsection{Subgradient update}

In this section, we prove Lemma~\ref{lem:Gordon-SE-GD-PR}, and also provide a technical lemma regarding Taylor expansions of the Gordon state evolution maps~\eqref{eq:Gordon-GD-PR-restated}. The latter lemma is used in the proof of Theorem~\ref{thm:GD-PR}(b).

\subsubsection{Proof of Lemma~\ref{lem:Gordon-SE-GD-PR}}

\apcomment{Insert after Gordon structure/notation stabilizes.}

\subsubsection{Perturbation lemma for Gordon state evolution maps}

\apcomment{Will modify by specializing to $\eta = 1/2$.}
\begin{lemma}[Local $\ell_\infty$ perturbation] \label{lem:Gordon-pert-GD}
Suppose the pair $(\xi, \sigma)$ satisfies $\xi/\sigma \geq 5$ and $\xi^2 + \sigma^2 \geq 0.9$. Also suppose that $\delta \geq 42$ and $\eta \leq 1/2$. There is a universal constant $\tau \in (0, 1)$ such that for all pairs of positive scalars $(\xi', \sigma')$ satisfying $|\xi' - \xi| \lor | \sigma' - \sigma| \leq 1/200$, we have
\begin{align*}
|F(\xi, \sigma) - F(\xi', \sigma')| &\leq (1 - \tau) \left( | \xi' - \xi| \lor |\sigma' - \sigma| \right) \text{ and } \\
|G(\xi, \sigma) - G(\xi', \sigma')| &\leq (1 - \tau) \left( | \xi' - \xi| \lor |\sigma' - \sigma| \right).
\end{align*}
\end{lemma}

\begin{proof}
First, let us restate the Gordon update as in equation~\eqref{eq:conv-rearrange} but for general stepsizes, with
\begin{align}
\sigmagordon &= \Big( (1 - 2\eta) \sigma^2 + (2\eta - 4\eta^2 / \delta) g^2 + \frac{4 \eta^2}{\delta} \Big\{ (\xi - f)^2 + (\sigma - g)^2 + (1 - f^2) + s^2 \Big\} \Big)^{1/2},
\end{align}
where $f = 1 - \frac{1}{\pi} (2 \alpha - \sin(2 \alpha))$ and $g = \frac{2}{\pi} \sin^2 \alpha$.
Also recall the interpolation $(\xi^u, \sigma^u) = u \cdot (\xi, \sigma) + (1 - u) \cdot (\xi', \sigma')$. Our analysis from before (cf. equation~\eqref{eq:Fmap-AMPR}) directly yields
\begin{align*}
\sup_{0 \leq u \leq 1} \| \nabla F (\xi^u, \sigma^u) \|_1 \leq \frac{\eta}{3 \pi} \sqrt{ \frac{2}{0.88} } + (1 - 2\eta) \leq 1 - 3\eta/ 2
\end{align*}
provided $\xi^2 + \sigma^2 \geq 0.9$ and $\sigma/\xi \leq 1/5$.

Turning now to the $G$ map, we have
\begin{align*}
\frac{\partial G}{\partial \sigma} \cdot 2G &= 2 (1 - 2\eta) \sigma + 2 \eta \cdot \frac{16}{\pi^2} \sin^3 \alpha \cos \alpha \cdot \left\{ -\xi / (\xi^2 + \sigma^2) \right\} \\
&\quad \quad+ \frac{4 \eta^2}{\delta} \left\{ 2 \sigma - 2\xi \frac{\partial f}{\partial \sigma} - 2 \sigma \frac{4}{\pi} \sin \alpha \cos \alpha \cdot \left\{ - \xi / (\xi^2 + \sigma^2) \right\} - \frac{4}{\pi} \sin^2 \alpha \right\}, \text{ and } \\
\frac{\partial G}{\partial \xi} \cdot 2G &= 2 \eta \cdot \frac{16}{\pi^2} \sin^3 \alpha \cos \alpha \cdot \left\{ \sigma / (\xi^2 + \sigma^2) \right\} \\
&\quad\quad + \frac{4 \eta^2}{\delta} \left\{ 2 \xi - 2\xi \frac{\partial f}{\partial \xi} - 2 f - 2 \sigma \frac{4}{\pi} \sin \alpha \cos \alpha \cdot \left\{ \sigma / (\xi^2 + \sigma^2) \right\} \right\}.
\end{align*}
Consequently, we have
\begin{align} 
\| \nabla G(\xi, \sigma) \|_1 G &\leq (1 - 2 \eta) \sigma + 2 \eta \cdot \frac{8}{\pi^2} \sin^3 \alpha \cdot \cos \alpha \cdot \sqrt{\frac{2}{\xi^2 + \sigma^2} } \notag \\
&\qquad + \frac{4 \eta^2}{\delta} \left( \xi \| \nabla f \|_1 + \sigma \cdot \frac{4}{\pi} \cdot \sin \alpha \cdot \cos \alpha \cdot \sqrt{ \frac{2}{\xi^2 + \sigma^2} } + | \sigma - g| + | \xi - f| \right) \notag \\
&\leq (1 - 2 \eta) \sigma + 2 \eta \cdot \frac{8}{\pi^2} \sin^3 \alpha \cdot \cos \alpha \cdot \frac{3}{2} \label{eq:key1} \\
&\qquad + \frac{4 \eta^2}{\delta} \left( \xi \cdot \frac{4}{\pi} \sin^2 \alpha \cdot \frac{3}{2} + \sigma \cdot \frac{4}{\pi} \cdot \sin \alpha \cdot \cos \alpha \cdot \frac{3}{2} + | \sigma - g| + | \xi - f| \right). \notag
\end{align}
%At the same time \apcomment{Transcribe from analysis above.}, we also have $f/g \geq \xi/\sigma$, so that for all $\xi \geq \sigma$, the rearrangement inequality yields $(\xi - g)^2 + (\sigma - f)^2 \leq (\xi - f)^2 + (\sigma - g)^2$. Thus,
%\begin{align} \label{eq:key2}
%G^2 \geq  (1 - 2\eta) \sigma^2_t + (2\eta - 4\eta^2 / \delta) g_t^2 + \frac{4 \eta^2}{\delta} \Big\{ (\xi - f)^2 + (\sigma - g)^2 + (1 - f^2) + s^2 \Big\}. 
%\end{align}
For two sequences $(a_n, b_n)_{n \geq 1}$ of positive reals, we have $(\sum_i a_i)^2 / \sum_{i} b_i \leq \sum_i a_i^2 b_i^{-1}$. Combining this with inequalities~\eqref{eq:conv-rearrange} and~\eqref{eq:key1}, we have
\begin{align*}
\| \nabla G(\xi, \sigma) \|_1^2 &\leq (1 - 2 \eta) \sigma + \frac{2\eta \delta}{\delta - 2 \eta} \cdot \left( \frac{64}{\pi^4} \sin^6 \alpha \cos^2 \alpha \cdot \frac{9}{4} \right) \div \left( \frac{4}{\pi^2} \sin^4 \alpha \right) \\
&\qquad \left( \frac{16 \eta^4 \xi^2}{\delta^2} \cdot \frac{144}{\pi^2} \sin^4 \alpha \right) \div \left( (2 \eta - 4\eta^2 / \delta ) \cdot \frac{4}{\pi^2} \sin^4 \alpha \right) + \frac{4 \eta^2}{\delta} \frac{(|\xi - f| + | \sigma - g|)^2}{(\xi - f)^2 + (\sigma - g)^2} \\
&\leq (1 - 2 \eta) \sigma + \frac{2\eta \delta}{\delta - 2 \eta} \cdot \frac{36}{25 \pi^2} + \frac{360 \eta^3}{\delta(\delta - 2\eta)} + \frac{8\eta^2}{\delta},
\end{align*}
where the last step holds for any $(\alpha, \xi)$ pair satisfying $\sin^2 (\alpha) \leq 1/25$ and $\xi \leq 1.05$. Moreover, $\sin^2 (\alpha^u) \leq 1/25$ and $\xi^u \leq 1.05$. Hence,
\begin{align*}
\sup_{0 \leq u \leq 1} \| \nabla G(\xi^u, \sigma^u) \|_1 \leq 0.98
\end{align*}
provided $\delta \geq C$.
% Putting this together with the bound~\eqref{eq:GD-PR-sigmaLB}, we have
% \begin{align*}
% \| \nabla G(\xi, \sigma) \|_1 &\leq \sqrt{1 - 2 \eta} \;\lor\; \sqrt{\eta} \cdot \frac{8}{\pi} \sin \alpha \cos \alpha \cdot \sqrt{\frac{1}{\xi^2 + \sigma^2}} \;\lor\; \frac{2\eta}{\sqrt{\delta}} \left( \xi \| \nabla f \|_1 + 2 \right).
% \end{align*}
% Now for large enough $\delta$ and $\eta \leq 1/2$, we have
% \begin{align*}
% \sup_{0 \leq u \leq 1} \| \nabla G(\xi^u, \sigma^u) \|_1 &\leq \sqrt{1 - 2\eta} \lor \sqrt{\eta} \leq 1 -\eta/2,
% \end{align*}
% provided the $(\xi, \sigma)$ pair satifies $\xi^2 + \sigma^2 \geq 0.9$ and $\sigma/\xi \leq 0.2$. 
\end{proof}
